# Supplementary material for: Influence of Pseudopotentials on Excitation Energies From Selected Configuration Interaction and Diffusion Monte Carlo
Source: arXiv:1904.00678 source file (2019-04-09)
Supplement: Supplementary file 1 [file ECP-SI.pdf]

# Supporting Information for "Influence of Pseudopotentials on Excitation Energies From Selected Configuration Interaction and Diffusion Monte Carlo"

Anthony Scemama,[1] Michel Caffarel,[1] Anouar Benali,[2] Denis Jacquemin,[3] and Pierre-François Loos[1, a)]

[1)] *Laboratoire de Chimie et Physique Quantiques, Université de Toulouse, CNRS, UPS, France*

[2)] *Computational Science Division, Argonne National Laboratory, Argonne, IL 60439, United States of America*

[3)] *Laboratoire CEISAM - UMR CNRS 6230, Université de Nantes, 2 Rue de la Houssinière, BP 92208, 44322 Nantes Cedex 3, France*

## I. GEOMETRIES

Below are given the cartesian coordinates of the water molecule investigated in this study. These are provided in atomic units (bohr) and they have been obtained at the CC3(full)/AVTZ level of theory.[1]

### A. Water

| | | | |
|---|---|---|---|
| O | 0.00000000 | 0.00000000 | -0.13209669 |
| H | 0.00000000 | 1.43152878 | 0.97970006 |
| H | 0.00000000 | -1.43152878 | 0.97970006 |

[1] P. F. Loos, A. Scemama, A. Blondel, Y. Garniron, M. Caffarel, and D. Jacquemin, J. Chem. Theory Comput. **14**, 4360 (2018).

[a)] Corresponding author: loos@irsamc.ups-tlse.fr

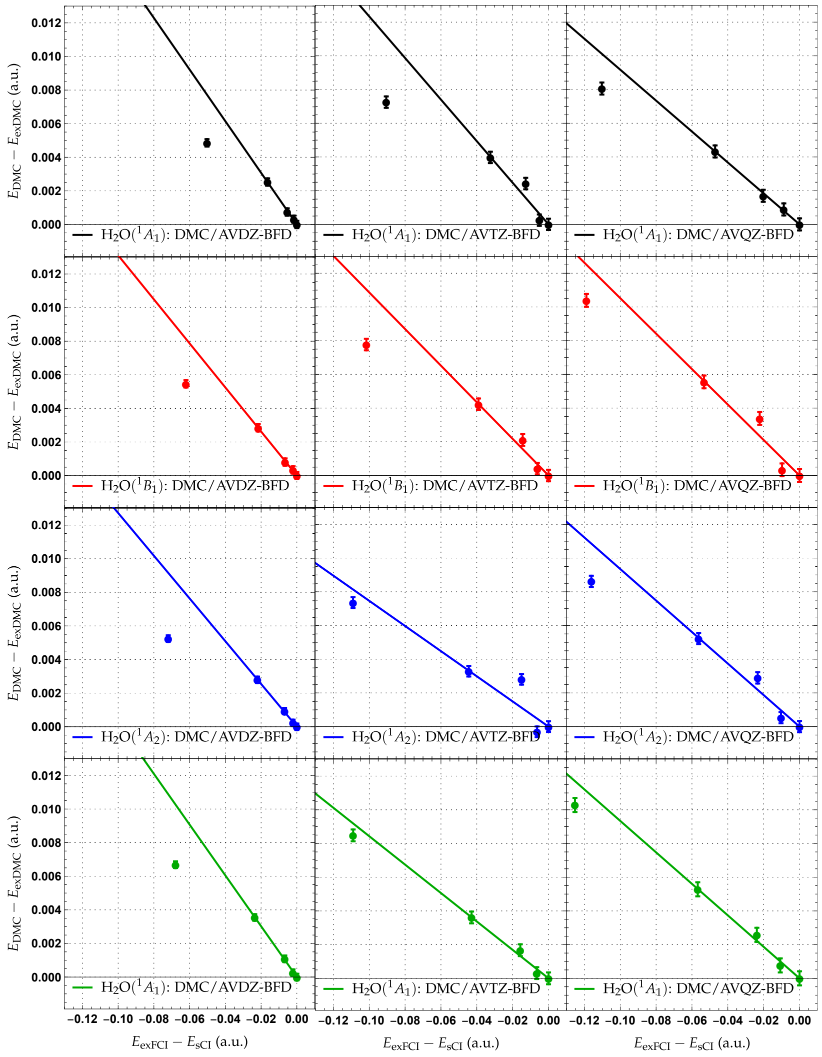


FIG. 1. Extrapolation of the FN-DMC energies for the singlet ground and excited states of the water molecule with the BFD pseudopotentials and the valence-only AVXZ basis sets (X = D, T, and Q). $E_{sCI}$ is the variational sCI energy, while $E_{exFCI}$ and $E_{exDMC}$ are the extrapolated sCI and FN-DMC energies, respectively. The last three points are taken into account in the linear extrapolation.

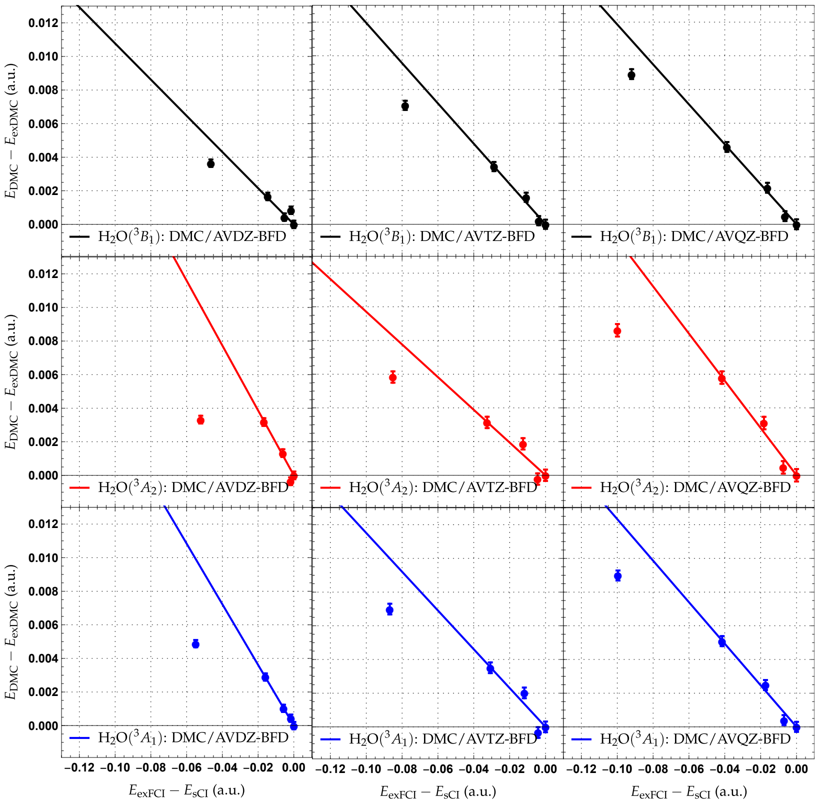


FIG. 2. Extrapolation of the FN-DMC energies for the triplet excited states of the water molecule with the BFD pseudopotentials and the valence-only AVXZ basis sets (X = D, T, and Q). $E_{\text{sCI}}$ is the variational sCI energy, $E_{\text{DMC}}$ is the FN-DMC energy, while $E_{\text{exFCI}}$ and $E_{\text{exDMC}}$ are the extrapolated sCI and FN-DMC energies, respectively. The last three points are taken into account in the linear extrapolation.
